# Supplementary material for: Inertial Collaborative Localisation for Autonomous Vehicles using a Minimum Energy Filter
Source: arXiv:2104.05897 source file (2021-04-13)
Supplement: Supplementary file 1 [file 8-appendix.tex]

\section{Appendix 1}
\red{
\begin{itemize}    
\item Derivative of the measurement function
\item Hessian of the Measurement function
\item Derivation of $E$, $A$ and $r$.
\end{itemize}
}
